# Supplementary material for: Beyond Faders: Understanding 6DoF Gesture Ecologies in Music Mixing
Source: arXiv:2602.23090 source file (2026-02-26)
Supplement: Supplementary file 1 [file Questionnaires.pdf]

## NASA-TLX

Place a dot at the scale that best indicates your experience of the task

**Mental Demand**

|  |  |  |  |  |  |  |  |  |  |
|--|--|--|--|--|--|--|--|--|--|
|  |  |  |  |  |  |  |  |  |  |
|--|--|--|--|--|--|--|--|--|--|

Low High

How much mental and perceptual activity was required (e.g. thinking, deciding, calculating, remembering, looking, searching, etc)? Was the task easy or demanding, simple or complex, exacting or forgiving?

**Physical Demand**

|  |  |  |  |  |  |  |  |  |  |
|--|--|--|--|--|--|--|--|--|--|
|  |  |  |  |  |  |  |  |  |  |
|--|--|--|--|--|--|--|--|--|--|

Low High

How much physical activity was required (e.g. pushing, pulling, turning, controlling, activating, etc)? Was the task easy or demanding, slow or brisk, slack or strenuous, restful or laborious?

**Temporal Demand**

|  |  |  |  |  |  |  |  |  |  |
|--|--|--|--|--|--|--|--|--|--|
|  |  |  |  |  |  |  |  |  |  |
|--|--|--|--|--|--|--|--|--|--|

Low High

How much time pressure did you feel due to the rate of pace at which the tasks or task elements occurred? Was the pace slow and leisurely or rapid and frantic?

**Performance**

|  |  |  |  |  |  |  |  |  |  |
|--|--|--|--|--|--|--|--|--|--|
|  |  |  |  |  |  |  |  |  |  |
|--|--|--|--|--|--|--|--|--|--|

Good Poor

How successful do you think you were in accomplishing the goals of the task set by the experimenter (or yourself)? How satisfied were you with your performance in accomplishing these goals?

**Effort**

|  |  |  |  |  |  |  |  |  |  |
|--|--|--|--|--|--|--|--|--|--|
|  |  |  |  |  |  |  |  |  |  |
|--|--|--|--|--|--|--|--|--|--|

Low High

How hard did you have to work (mentally and physically) to accomplish your level of performance?

**Frustration**

|  |  |  |  |  |  |  |  |  |  |
|--|--|--|--|--|--|--|--|--|--|
|  |  |  |  |  |  |  |  |  |  |
|--|--|--|--|--|--|--|--|--|--|

Low High

How insecure, discouraged, irritated, stressed and annoyed versus secure, gratified, content, relaxed and complacent did you feel during the task?

## UEQ

Mark the circle that best indicates your experience of the prototype

### English version

|                 |               |              |
|-----------------|---------------|--------------|
| obstructive     | o o o o o o o | supportive   |
| complicated     | o o o o o o o | easy         |
| inefficient     | o o o o o o o | efficient    |
| confusing       | o o o o o o o | clear        |
| boring          | o o o o o o o | exciting     |
| not interesting | o o o o o o o | interesting  |
| conventional    | o o o o o o o | inventive    |
| usual           | o o o o o o o | leading edge |
