# Supplementary material for: Beyond Faders: Understanding 6DoF Gesture Ecologies in Music Mixing
Source: arXiv:2602.23090 source file (2026-02-26)
Supplement: Supplementary file 2 [file participants_recruitment_form.pdf]

# HCI2000 Call for Participants

We are DLSU Computer Science students conducting research entitled "**Gestures for Immersive Music Mixing**".

We are looking for participants who have **no experience in music mixing**, where they have **never used a digital audio workstation** (e.g., FL Studio, Ableton Live, etc.) **and a mixing console**. Participants will be part of a **one day user study** that will take **at most 1 hours**.

You will be **using a VR headset** to see your hand gesture preferences in controlling certain sound elements.

The date will be **based on participant's availability**. We will be asking for your **availability from October 20 to November 7**. This will take place in **De La Salle University Manila**.

There are no right or wrong answers, and no judgments will be made during the user study. We are here to learn from your thoughts and preferences.

**Confidentiality Notice:** All responses and data will be treated with strict confidentiality and used solely for academic research purposes. *Your data will be treated with the utmost confidentiality and will only be used for the purposes of our research. We will anonymize your data making sure it cannot be traced to you. We are committed to ensuring that no information will be shared or leaked outside of academic purposes.*

---

\* Indicates required question

1. Email \*

---

## Data Privacy and Consent Form

We, the researchers, respect your privacy and are committed to complying with the Data Privacy Act of 2012. Please read this form carefully before providing your personal information and input.

### Purpose of Data Collection:

By filling out this form, you agree that your personal data, including but not limited to your name, contact details, and insights provided during this research, will be used for the following purposes:

- To log and track your participation in our research.
- To contact you for future communication related to this study.
- To analyze and assess the feedback and insights you provide for the purpose of validating the training lessons for our thesis project on *Exploring the Use of AR Piano Roll Visualizations in Teaching Blues Improvisation*.

### Confidentiality:

We assure you that:

- All personal data and information you provide will be treated with strict confidentiality and will not be shared with anyone outside of the research team.
- Your data will be used **solely** for the purposes of our study.
- No personal identifiers will be included in the final report or publications arising from this study. All data will be anonymized.

### Data Retention:

Your personal data will be securely stored for the duration of our research project. Once our study is complete:

- Data will be retained for internal records until the completion of our research project, after which it will be securely deleted, unless otherwise requested.
- You may request for your data to be deleted by contacting us.

### By consenting, you acknowledge and agree that:

- Your insights and data will be used for this study.
- Your personal data will be used for contact and logging purposes.
- Your personal information will remain confidential.
- You may request the deletion of your personal data.

## 2. Do you consent? \*

*Mark only one oval.*

☐ I have read and understood the information provided in this form, and I voluntarily and willingly consent to participate in the study.

☐ I do not consent to participate in the study.

**Background**

## 3. Name (Surname, Firstname) \*

Ex. Dela Cruz, Juan

---

## 4. Contact Number \*

Ex. 0917XXXXXXX

---

## 5. Facebook or Messenger Link \*

Ex. <https://www.facebook.com/username>

---

## 6. Do you have any experience in using a digital audio workstation (DAW)? \*

*Mark only one oval.*

☐ Yes

☐ No

7. Do you have any experience in using a mixing console? \*

*Mark only one oval.*

☐ Yes

☐ No

8. Do you have any experience in using a music production? \*

*Mark only one oval.*

☐ Yes

☐ No

9. Which weekdays are you available between October 20 to October 31? (From 9am-6pm) \*

---

---

---

---

---

Thank you for your interest!

Thank you for showing interest in participating in our study. Your thoughts and feedback will play a crucial role in shaping the success of our research, and we greatly appreciate your willingness to contribute.

Should you have any questions, clarifications, or concerns, please feel free to reach out to us at any time. You can contact us via Facebook, and we will be more than happy to assist you. **Jeremy Chen** Messenger: [www.facebook.com/jremy.chen](https://www.facebook.com/jremy.chen) **Rendell Ngo** Messenger: [www.facebook.com/rendell.ngo](https://www.facebook.com/rendell.ngo) **Ethan Badayos** Messenger: [www.facebook.com/ethan.romey](https://www.facebook.com/ethan.romey) **Hans Lumagui** Messenger: [www.facebook.com/hans.lumagui.2024](https://www.facebook.com/hans.lumagui.2024)
